# Supplementary material for: Zinc Electrode Shape-Change in Secondary Air Batteries: A 2D Modeling Approach
Source: arXiv:1903.00382 ancillary file (2019-03-01)
Supplement: Supplementary file 1 [file Supplementary_Information.pdf]

# Supplementary Materials for Zinc Electrode Shape-Change in Secondary Air Batteries: A 2D Modeling Approach

Tobias Schmitt[a,b,c], Tobias Arlt[d], Ingo Manke[e], Arnulf Latz[a,b,c], Birger Horstmann[a,b,c,*]

[a] *German Aerospace Center, Pfaffenwaldring 38-40, 70569 Stuttgart, Germany*
[b] *Helmholtz Institute Ulm, Helmholtzstraße 11, 89069 Ulm, Germany*
[c] *Ulm University, Institute of Electrochemistry, Albert-Einstein-Allee 47, 89069 Ulm, Germany*
[d] *Technical University of Berlin, Material Sciences and Technology, Hardenbergstraße 36, 10623 Berlin, Germany*
[e] *Helmholtz Center for Materials and Energy, Hahn-Meitner-Platz 1, 14109 Berlin, Germany*

---

---

**Contents**

**S1 Experimental Setup** 2

**S2 Solid Phase Parameters** 2
S2.1 Zinc Anode Morphology . . . . . 2
S2.2 Conductivity . . . . . 4
S2.3 Leverett Function (Solid) . . . . . 5
S2.4 Tortuosity / Effective Transport Tensor . . . . . 5

**S3 Liquid Phase Parameters** 5
S3.1 Chemical Potentials . . . . . 6
S3.2 Partial Molar Volumes . . . . . 6
S3.3 Diffusion Coefficients . . . . . 7
S3.4 Conductivity . . . . . 7
S3.5 Transference Numbers . . . . . 8
S3.6 Permeability . . . . . 8
S3.7 Viscosity . . . . . 8
S3.8 Leverett Function (Liquid) . . . . . 9

**S4 Reactions and Parameters** 9
S4.1 Reaction I: Zinc Dissolution and Deposition . . . . . 9
S4.2 Reaction II: Zinc Oxide Precipitation . . . . . 10
S4.3 Reaction III: Oxygen Dissolution . . . . . 10
S4.4 Reaction IV: Oxygen Reduction and Evolution . . . . . 11
S4.5 Reaction V: Carbonation . . . . . 11

**S5 Validation of Implementation: 1D vs. 3D** 12

**S6 Determination of Optimal Grid Resolution** 12

**S7 Solid Phase Movement** 12

*Corresponding author
*URL:* `birger.horstmann@dlr.de` (Birger Horstmann)

**S8 Reaction and Transport Kinetics Optimization** **14**

## S1. Experimental Setup

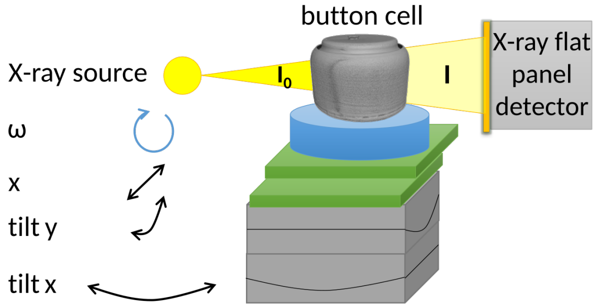


Figure S1: Experimental set-up: "tilt x" and "tilt y" is used to adjust the rotation axis; x-translation table; $\omega$-rotation table; $I_0$ - initial X-ray beam. Reproduced from Ref. [1] with permission from the PCCP Owner Societies.

## S2. Solid Phase Parameters

### *S2.1. Zinc Anode Morphology*

In Sections 3.2 and 3.5, we describe our model for the zinc anode morphology and our reaction theory. In order to accurately describe the reaction source rates $\mathring{\mathcal{P}}^{\Theta}$, we have to specify the anode morphology and the specific surface areas. We model the anode by spherically symmetric primitive particles (see Figs. 2 and S2a). Each of these particles consists of a zinc core with radius $r_{Zn}$ and a porous zinc oxide shell with radius $r_{ZnO}$. This porous layer acts as diffusion barrier for hydroxide ions slowing down their diffusion from the bulk electrolyte to the zinc surface. This in turn affects the dissolution of metallic zinc.

We model this morphology with three independent variables, the zinc volume fraction $\varepsilon_{Zn}$, the zinc oxide volume fraction $\varepsilon_{ZnO}$, and the density of primitive particles $\left\langle \mathcal{N}_{pp} \right\rangle$ (see Eq. (13)). The following derivation uses an arbitrary volume $V$. Going beyond our previous work in Ref. [2], we take into account the overlap of primitive particles as depicted in Fig. S2b.

The surface of a single zinc particle is given by

$$A'_{Zn} = 4\pi r_{Zn}^2 \, . \tag{S1}$$

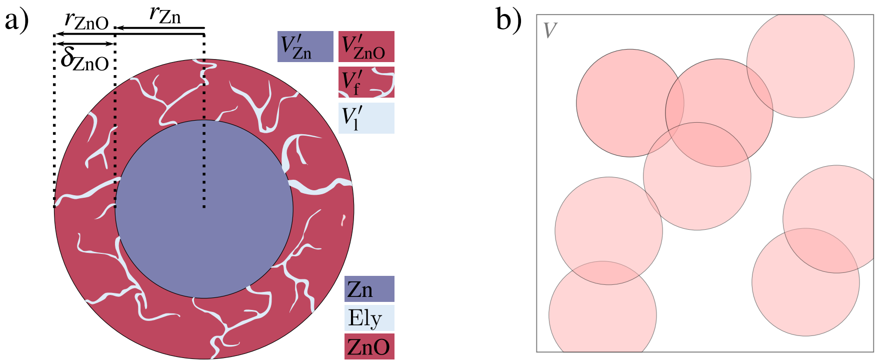


Figure S2: (a) Modeling of the anode structure by spherically symmetric objects (primitive particles). They consist of a zinc core and a porous zinc oxide shell filled with electrolyte (motivated by Ref. [3]). Apostrophes mark the volumes of a single primitive particle. (b) Cross section of the anode material. It consists of overlapping spherical primitive Zn / ZnO particles.

We sum up the volumes of $N_{\mathrm{pp}}$ individual primitive particles $V_{\mathrm{P}} = V_1 = \cdots = V_{N_{\mathrm{pp}}}$ and subtract the overlap. To take care of multiple overlap, we add that one again. Carrying on this consideration results in

$$\varepsilon_{\mathrm{Zn}} V = \left(V_1 + \cdots + V_{N_{\mathrm{pp}}}\right) - (\varepsilon_{\mathrm{Zn}})\left(V_1 + \cdots + V_{N_{\mathrm{pp}}}\right) + (\varepsilon_{\mathrm{Zn}})^2\left(V_1 + \cdots + V_{N_{\mathrm{pp}}}\right) - \cdots = N_{\mathrm{pp}} V_{\mathrm{P}} \sum_{i=0}^{\infty} (-\varepsilon_{\mathrm{Zn}})^i \,. \tag{S2}$$

The first part of Eq. (S2) sums up all primitive particles. The second one subtracts the overlap of the particles, whereas the third part corrects again the multiple subtraction of the same region. This iteration yields a geometric series resulting in

$$\varepsilon_{\mathrm{Zn}} = \left\langle \mathcal{N}_{\mathrm{pp}} \right\rangle V_{\mathrm{P}} \frac{1}{1 + \varepsilon_{\mathrm{Zn}}} \,, \tag{S3}$$

with $\left\langle \mathcal{N}_{\mathrm{pp}} \right\rangle = N_{\mathrm{pp}}/V$. Expressing $V_{\mathrm{P}}$ by its radius, Eq. (S3) is written as

$$\left\langle \mathcal{N}_{\mathrm{pp}} \right\rangle \frac{4\pi}{3} r_{\mathrm{Zn}}^3 \frac{1}{1 + \varepsilon_{\mathrm{Zn}}} = \varepsilon_{\mathrm{Zn}} \,. \tag{S4}$$

Using the initial values $r_{\mathrm{Zn}}^0$ and $\varepsilon_{\mathrm{Zn}}^0$ yields the initial density of primitive particles

$$\left\langle \mathcal{N}_{\mathrm{pp}} \right\rangle^0 = \frac{3}{4\pi} \varepsilon_{\mathrm{Zn}}^0 (1 + \varepsilon_{\mathrm{Zn}}^0) \frac{1}{(r_{\mathrm{Zn}}^0)^3} \,. \tag{S5}$$

The initial radius $r_{\mathrm{Zn}}^0 = 35\,\mu\mathrm{m}$ of the zinc particles is extracted from SEM images and tomographies [4]. The radius of the particles is

$$r_{\mathrm{Zn}} = \left[ \frac{3}{4\pi} \frac{\varepsilon_{\mathrm{Zn}}(1 + \varepsilon_{\mathrm{Zn}})}{\left\langle \mathcal{N}_{\mathrm{pp}} \right\rangle} \right]^{\frac{1}{3}} \,. \tag{S6}$$

This results in a specific effective zinc surface area

$$A_{\mathrm{Zn}} = \left\langle \mathcal{N}_{\mathrm{pp}} \right\rangle a_{\mathrm{Zn}} 4\pi r_{\mathrm{Zn}}^2 (1 - \varepsilon_{\mathrm{Zn}}) \,. \tag{S7}$$

With the term $(1 - \varepsilon_{\mathrm{Zn}})$, we take into account the overlap of primitive particles.

SEM images by Horn et al. show that the zinc oxide is formed as a porous layer around the zinc particles [3]. For simplicity, we assume that the shell forms directly on the zinc surface. Therefore, the inner radius of the passivation shell is $r_{\mathrm{Zn}}$. As shown in Fig. S2a, the total volume $V_{\mathrm{f}}$ of the shell is made up of the zinc oxide volume $V'_{\mathrm{ZnO}}$ and electrolyte filled pores with volume $V'_{\mathrm{l}}$,

$$V'_{\mathrm{f}} = V'_{\mathrm{ZnO}} + V'_{\mathrm{l}} \,. \tag{S8}$$

With the solid volume fraction $\varepsilon_{\mathrm{f}}$ of the shell, we can write

$$V'_{\mathrm{ZnO}} = \varepsilon_{\mathrm{f}} V'_{\mathrm{f}} \,, \qquad V'_{\mathrm{l}} = (1 - \varepsilon_{\mathrm{f}}) V'_{\mathrm{f}} \,. \tag{S9}$$

The volume of a spherical shell is $V_{\mathrm{f}} = 4\pi/3 \left((r_{\mathrm{ZnO}})^3 - (r_{\mathrm{Zn}})^3\right)$. The derivation of the effective surface area for zinc oxide is analogous to the one for zinc. The total zinc oxide volume is

$$\left\langle \mathcal{N}_{\mathrm{pp}} \right\rangle V'_{\mathrm{ZnO}} \frac{1}{1 + \varepsilon_{\mathrm{ZnO}}} = \varepsilon_{\mathrm{ZnO}} \,. \tag{S10}$$

Thus, the outer radius $r_{\mathrm{ZnO}}$ is

$$r_{\mathrm{ZnO}} = \left[ \frac{3}{4\pi} \frac{\varepsilon_{\mathrm{ZnO}}(1 + \varepsilon_{\mathrm{ZnO}})}{\varepsilon_{\mathrm{f}} \left\langle \mathcal{N}_{\mathrm{pp}} \right\rangle} + r_{\mathrm{Zn}}^3 \right]^{\frac{1}{3}} \,. \tag{S11}$$

This results in a specific effective surface area of the zinc oxide of

$$A_{\mathrm{ZnO}} = 2 \cdot \left\langle N_{\mathrm{pp}} \right\rangle 4\pi \left(r_{\mathrm{ZnO}}\right)^2 \left(1 - \varepsilon_{\mathrm{ZnO}}\right) \tag{S12}$$

for a shell thickness of $\delta_{\mathrm{ZnO}} = r_{\mathrm{ZnO}} - r_{\mathrm{Zn}}$. The 2 encodes that ZnO formation takes place not only at the outer shell surface, but also on the inner shell surface and inside the porous structure.

Now, we can enlist the specific surface areas for all reactions (see Section S4). These are

$$A_{\mathrm{I}} = A_{\mathrm{l,Zn}}\,,$$

$$A_{\mathrm{II}} = \begin{cases} 0 & \text{if } (c_{\mathrm{Zn(OH)_4^{2-}}} \leq c_{\mathrm{crit}}) \text{ and } (j_{\mathrm{II}} \geq 0) \\ f_{\mathrm{nuc}}(\varepsilon_{\mathrm{ZnO}}) \cdot A_{\mathrm{l,ZnO}} & \text{else}\,, \end{cases}$$

$$A_{\mathrm{III}} = A_{\mathrm{l,g}} = 3 \cdot 10^2\,\frac{\mathrm{m}^2}{\mathrm{m}^3}\,, \tag{S13}$$

$$A_{\mathrm{IV}} = A_{\mathrm{l,GDE}} = 1 \cdot 10^3\,\frac{\mathrm{m}^2}{\mathrm{m}^3}\,, \tag{S14}$$

$$A_{\mathrm{V}} = A_{\mathrm{l,g}} = 3 \cdot 10^2\,\frac{\mathrm{m}^2}{\mathrm{m}^3}\,. \tag{S15}$$

Here, the interfaces $A_{\mathrm{l,Zn}} = A_{\mathrm{Zn}}$ and $A_{\mathrm{l,ZnO}} = A_{\mathrm{ZnO}}$ are determined by the morphology model from above in Eq. (S7) and Eq. (S12), respectively.

The critical concentration $c_{\mathrm{crit}}$ is discussed together with our model for zinc oxide nucleation in Section S4.2. The function $f_{\mathrm{nuc}}(\varepsilon_{\mathrm{ZnO}})$ is our numeric implementation of the nucleation of zinc oxide [2]. We assume that the surface $A_{\mathrm{II}}$ grows slowly from zero to its final value for very small values of $\varepsilon_{\mathrm{ZnO}}$. In order to ensure a continuous differentiable smoothing function, we use

$$f_{\mathrm{nuc}}(\varepsilon_{\mathrm{ZnO}}) = \begin{cases} \sin\left(\frac{\pi}{2}\frac{\varepsilon_{\mathrm{ZnO}}}{\varepsilon_{\mathrm{ZnO}}^{\mathrm{crit}}}\right) & \text{if } \varepsilon_{\mathrm{ZnO}} < \varepsilon_{\mathrm{ZnO}}^{\mathrm{crit}} \\ 1 & \text{else.} \end{cases} \tag{S16}$$

The value of $\varepsilon_{\mathrm{ZnO}}^{\mathrm{crit}}$ is determined by the critical thickness $\delta_{\mathrm{crit}}$ at which the full surface is formed. For small zinc oxide volume fractions $\varepsilon_{\mathrm{ZnO}}$, we can Taylor expand the expressions for the radii in Eq. (S6) and in Eq. (S11)

$$\delta_{\mathrm{crit}} = r_{\mathrm{ZnO}} - r_{\mathrm{Zn}} \approx r_{\mathrm{Zn}}^0 \left[3\,\frac{\varepsilon_{\mathrm{ZnO}}}{\varepsilon_{\mathrm{f}}\varepsilon_{\mathrm{Zn}}^0}\right]. \tag{S17}$$

Rearranging the terms, yields the critical zinc oxide volume fraction $\varepsilon_{\mathrm{ZnO}}^{\mathrm{crit}} = 3\varepsilon_{\mathrm{f}}\varepsilon_{\mathrm{Zn}}^0\delta_{\mathrm{crit}}/r_{\mathrm{Zn}}^0$. We set the critical thickness to $\delta_{\mathrm{crit}} = 6.5083 \cdot 10^{-8}$ m, which corresponds to 125 times the lattice constant of zinc oxide.

In the design optimizations of Section 6.1, we model a supporting structure. This guarantees a minimum surface, on which zinc and zinc oxide can precipitate. For simplicity, we assume that some zinc metal cannot dissolve. In reality, one would choose a different material for the supporting structure. We assume a minimum zinc volume fraction of $\varepsilon_{\mathrm{Zn,min}} = 0.019$ and a minimum specific surface area of $\sim 4.3 \cdot 10^3\ \mathrm{m}^{-1}$.

### *S2.2. Conductivity*

The solid conductivity $\kappa_{\mathrm{s}}$ depends on the material [5, 6]. Its values are listed in Table S1. The total conductivity of the anode material is calculated by

$$\kappa_{\mathrm{s}} = \frac{\varepsilon_{\mathrm{Zn}}\kappa_{\mathrm{Zn}} + \varepsilon_{\mathrm{ZnO}}\kappa_{\mathrm{ZnO}} + \varepsilon_{\mathrm{P}}\kappa_{\mathrm{PA}}}{\varepsilon_{\mathrm{Zn}} + \varepsilon_{\mathrm{ZnO}} + \varepsilon_{\mathrm{P}}}\,. \tag{S18}$$

Knowledge on electrode micro-structure and Zn metal content in ZnO shell would allow an improved parameterization of solid conductivity. We have checked numerically that the details of the volume-averaged solid conductivity hardly affect zinc-air battery cycling.

| Coefficient | Value in $\left[\frac{\mathrm{S}}{\mathrm{m}}\right]$ |
|---|---|
| $\kappa_{\mathrm{Zn}}$ | $1.66 \cdot 10^{7}$ |
| $\kappa_{\mathrm{ZnO}}$ | $4.6 \cdot 10^{-1}$ |
| $\kappa_{\mathrm{PA}}$ | $5.85 \cdot 10^{7}$ |
| $\kappa_{\mathrm{Sep}}$ | 0 |
| $\kappa_{\mathrm{GDE}}$ | $1 \cdot 10^{4}$ |
| $\kappa_{\mathrm{CC}}$ | $2 \cdot 10^{6}$ |

Table S1: Conductivity of the solid phases. The abbreviations are: passive material anode (PA), separator (Sep), gas diffusion electrode (GDE), and current collector (CC).

### *S2.3. Leverett Function (Solid)*

Our novel model for convection of the solid phase relies on a pseudo-pressure calculated with a Leverett-like function (see Section 3.2). We assume that the solid volume expansion either densifies the phase or induces a convection. The latter is described by a pseudo-pressure $\overline{p}_{\mathrm{s}}$. The separation of both effects is regulated by a threshold $s_{\mathrm{s}}^{*}$ for the solid saturation $s_{\mathrm{s}} = (\varepsilon_{\mathrm{Zn}} + \varepsilon_{\mathrm{ZnO}})/(1 - \varepsilon_{\mathrm{P}})$. The solid Leverett function is

$$J_{\mathrm{s}}(s_{\mathrm{s}}) = \begin{cases} 0 & \text{if } s_{\mathrm{s}} < s_{\mathrm{s}}^{*} \\ \left[c_1\,(s_{\mathrm{s}} - s_{\mathrm{s}}^{*})\right]^{c_2} & \text{else} \end{cases} \tag{S19}$$

with $c_1 = 0.01$, $c_2 = 2$, and if not stated differently $s_{\mathrm{s}}^{*} = 0.8$. The pseudo-permeability $\omega$ in the calculation of the solid velocity is set to $\omega = 1 \cdot 10^{-6}\,\mathrm{m}^2{\cdot}\mathrm{Pa}^{-1}{\cdot}\mathrm{s}^{-1}$.

### *S2.4. Tortuosity / Effective Transport Tensor*

We assume a macroscopically isotropic phase distribution. This reduces the effective transport tensor to one degree of freedom. Thus, it is expressed by a scalar tortuosity factor $\boldsymbol{T}_{\alpha}^{\mathrm{eff}} \approx \boldsymbol{I}/\tau_{\alpha}$, with the tortuosity $\tau_{\alpha}$. In this case, we can drop the identity matrix $\boldsymbol{I}$. The tortuosity itself is modeled with a Bruggemann coefficient b and is only dependent on the volume fraction

$$\tau_{\alpha} = \frac{1}{\varepsilon_{\alpha}^{\mathrm{b}-1}}\,. \tag{S20}$$

If not stated differently, we use b = 1.5.

## S3. Liquid Phase Parameters

Here, we enlist the parameters for electrolyte transport modeled in Section 3.3. We present all parameters in their general form ($D_{\beta_{\mathrm{l}}}$, not $\overline{D}_{\beta_{\mathrm{l}}}$). An intrinsic average is obtained by a calculation with the intrinsic averaged arguments, for example,

$$\begin{aligned} D_{\mathrm{OH^-}} &= D_{\mathrm{OH^-}}(c_{\mathrm{OH^-}}, c_{\mathrm{Zn(OH)_4^{2-}}}, T)\,, \\ \overline{D}_{\mathrm{OH^-}} &\approx D_{\mathrm{OH^-}}(\overline{c}_{\mathrm{OH^-}}, \overline{c}_{\mathrm{Zn(OH)_4^{2-}}}, \overline{T})\,. \end{aligned}$$

The definitions of the standard concentrations are

$$c_{\mathrm{std}} = 1 \cdot 10^{3}\,\frac{\mathrm{mol}}{\mathrm{m}^3}\,, \qquad c_{\mathrm{std}}^{\mathrm{O_2}} = 1.42 \cdot 10^{-2}\,\frac{\mathrm{mol}}{\mathrm{m}^3}\,. \tag{S21}$$

*S3.1. Chemical Potentials*

We use the chemical potentials of ideal mixtures $\mu_{\beta_1} = \mu^0_{\beta_1} + RT \ln \frac{c_{\beta_1}}{c_{\mathrm{std}}}$, with the chemical potentials at standard conditions $\mu^0_{\beta_1}$. The constant chemical potentials at standard condition $\mu^0_{\beta_1}$ determine the reaction free energy, but vanish in derivatives of $\mu_{\beta_1}$. Thus, the thermodynamic factor for the transport equations in Eq. (22) is

$$\frac{\partial \mu_{\beta_1}}{\partial c_{\beta_1}} = \frac{RT}{c_{\beta_1}} . \tag{S22}$$

*S3.2. Partial Molar Volumes*

The measured partial molar volumes for an aqueous solution of hydroxide and zinc oxide are given in Ref. [7]. As discussed by Stamm et al. [2], the system of $H_2O$, $OH^-$, $Zn(OH)_4^{2-}$, $CO_3^{2-}$, $O_2^{\mathrm{l}}$ is transformed to the one of Ref. [7] by

$$\begin{aligned} c_1 &= c_{H_2O} + c_{Zn(OH)_4^{2-}} , \\ c_2 &= c_{OH^-} + 2c_{Zn(OH)_4^{2-}} + 2c_{CO_3^{2-}} , \\ c_3 &= c_{Zn(OH)_4^{2-}} . \end{aligned} \tag{S23}$$

We fit the calculations of Ref. [2] with a polynomial dependent on the three independent variables $c_1$, $c_2$ and $c_3$. The results are shown in Fig. S3. The fit function has the form

$$v = A + B_1c_1 + B_2c_2 + B_3c_3 + D_1c_1^2 + D_2c_2^2 + D_3c_3^2 + D_4c_1c_2 + D_5c_1c_3 + D_6c_2c_3 + E_1c_1c_2c_3 . \tag{S24}$$

The coefficients of Eq. (S24) are listed in Table S2. For carbonate and oxygen, we use [8]

$$v_{K_2CO_3} = 8.217 \cdot 10^{-5} \frac{\mathrm{m}^3}{\mathrm{mol}} \qquad v_{O_2^{\mathrm{l}}} = 3.32 \cdot 10^{-5} \frac{\mathrm{m}^3}{\mathrm{mol}} \tag{S25}$$

| | $H_2O$ | KOH | $K_2Zn(OH)_4$ |
|---|---|---|---|
| $A$ / $\frac{\mathrm{m}^3}{\mathrm{mol}}$ | $1.8175 \cdot 10^{-5}$ | $1.4856 \cdot 10^{-5}$ | $5.7272 \cdot 10^{-5}$ |
| $B_1$ / $\frac{\mathrm{m}^6}{\mathrm{mol}^2}$ | $-1.2345 \cdot 10^{-12}$ | $-1.3543 \cdot 10^{-10}$ | $-5.1708 \cdot 10^{-10}$ |
| $B_2$ / $\frac{\mathrm{m}^6}{\mathrm{mol}^2}$ | $-2.2671 \cdot 10^{-10}$ | $2.2820 \cdot 10^{-9}$ | $6.7650 \cdot 10^{-9}$ |
| $B_3$ / $\frac{\mathrm{m}^6}{\mathrm{mol}^2}$ | $-4.9118 \cdot 10^{-10}$ | $1.8299 \cdot 10^{-9}$ | $1.5825 \cdot 10^{-7}$ |
| $D_1$ / $\frac{\mathrm{m}^9}{\mathrm{mol}^3}$ | 0.0 | $6.9007 \cdot 10^{-16}$ | $2.4885 \cdot 10^{-15}$ |
| $D_2$ / $\frac{\mathrm{m}^9}{\mathrm{mol}^3}$ | 0.0 | $-8.5313 \cdot 10^{-14}$ | $-2.5503 \cdot 10^{-13}$ |
| $D_3$ / $\frac{\mathrm{m}^9}{\mathrm{mol}^3}$ | 0.0 | $-3.2479 \cdot 10^{-13}$ | $-1.5842 \cdot 10^{-12}$ |
| $D_4$ / $\frac{\mathrm{m}^9}{\mathrm{mol}^3}$ | $2.5577 \cdot 10^{-15}$ | $-7.0756 \cdot 10^{-15}$ | $-1.3967 \cdot 10^{-14}$ |
| $D_5$ / $\frac{\mathrm{m}^9}{\mathrm{mol}^3}$ | $5.5114 \cdot 10^{-15}$ | $9.7373 \cdot 10^{-15}$ | $-2.5197 \cdot 10^{-14}$ |
| $D_6$ / $\frac{\mathrm{m}^9}{\mathrm{mol}^3}$ | $4.4817 \cdot 10^{-14}$ | $-1.7543 \cdot 10^{-13}$ | $-1.3482 \cdot 10^{-12}$ |
| $E$ / $\frac{\mathrm{m}^{12}}{\mathrm{mol}^4}$ | $-6.7216 \cdot 10^{-19}$ | $4.1464 \cdot 10^{-19}$ | $8.9193 \cdot 10^{-18}$ |

Table S2: Coefficients of the fit function Eq. (S24) for the partial molar volumes.

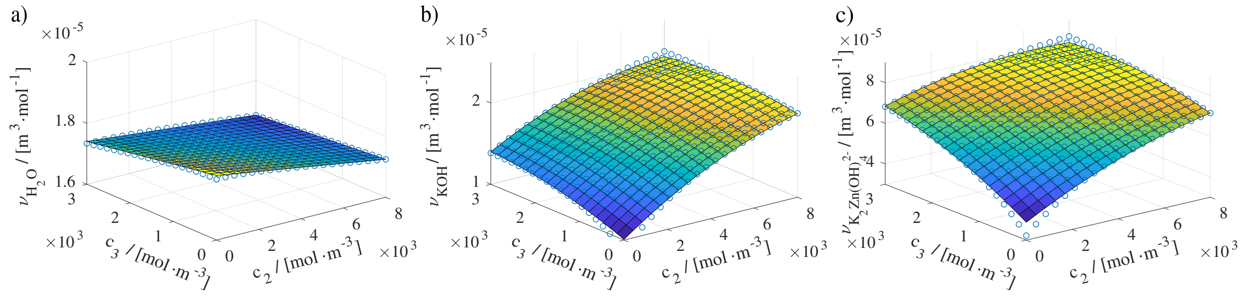


Figure S3: Fitted partial molar volumes in an aqueous potassium hydroxide solution for water (a), potassium hydroxide (b), and zincate (c). Light blue circles represent the data points, originating from Ref. [2], with the fit function as colored surface plot. $c_1$ is fixed in the plots to $46 \cdot 10^3$ mol·m$^{-3}$.

### *S3.3. Diffusion Coefficients*

The diffusion coefficient of hydroxide ions in a potassium hydroxide solution is $D_{OH^-} = 3.5 \cdot 10^{-10}\,\frac{m^2}{s}$ [9]. The zincate diffusion coefficient was determines by May et al. [10] as

$$D_{Zn(OH)_4^{2-}} = -9.33 \cdot 10^{-11}\,\frac{m^2}{s}\frac{c_{K^+}}{c_{std}} + 12 \cdot 10^{-10}\,\frac{m^2}{s}\,. \tag{S26}$$

The ones of carbon dioxide and carbonate are obtained from Ref. [11, 12]. They are $D_{CO_2} = 1.5 \cdot 10^{-9}\,\frac{m^2}{s}$ and $D_{CO_3^{2-}} = 8.2 \cdot 10^{-10}\,\frac{m^2}{s}$. The diffusion coefficient of oxygen was measured by Davis et al. [13]. Stamm et al. fit an exponential function to it [2] which results in

$$D_{O_2} = 1.5 \cdot 10^{-9}\,\frac{m^2}{s} \cdot \exp\left(-0.2878\frac{c_{K^+}}{c_{std}}\right) + 4 \cdot 10^{-10}\,\frac{m^2}{s}\,. \tag{S27}$$

### *S3.4. Conductivity*

| Coefficient | Value | Units |
|---|---|---|
| $K_1$ | $2.798 \cdot 10^{1}$ | $\left[\frac{S}{m}\right]$ |
| $K_2$ | $-9.241 \cdot 10^{-1}$ | $\left[\frac{S}{m \cdot K}\right]$ |
| $K_3$ | $-1.496 \cdot 10^{-2}$ | $\left[\frac{S}{m \cdot K^2}\right]$ |
| $K_4$ | $-9.052 \cdot 10^{-2}$ | $\left[\frac{S}{m \cdot K}\right]$ |
| $K_5$ | $1.149 \cdot 10^{-2}$ | $\left[\frac{S}{m \cdot K^2}\right]$ |
| $K_6$ | $1.765 \cdot 10^{-1}$ | [1] |
| $K_7$ | $6.966 \cdot 10^{0}$ | $\left[\frac{S}{m \cdot K}\right]$ |
| $K_8$ | $-2.898 \cdot 10^{3}$ | $\left[\frac{S \cdot K}{m}\right]$ |

Table S3: Fit coefficients of $\kappa_{KOH}$ of Eq. (S30). The values are obtained from Ref. [14].

Liu et al. determine the conductivity $\kappa_l$ of a potassium hydroxide solution [15], which is calculated with a linear mixture rule

$$\kappa_l = \Lambda_{KOH} c_{OH^-} + 2\Lambda_{K_2Zn(OH)_4} c_{Zn(OH)_4^{2-}} + 2\Lambda_{K_2CO_3} c_{CO_3^{2-}}\,. \tag{S28}$$

The equivalent conductivity of binary potassium hydroxide is $\Lambda_{\mathrm{KOH}} = \kappa_{\mathrm{KOH}}/c_{\mathrm{K^+}}$. The ones of zincate and carbonate are

$$\Lambda_{\mathrm{K_2Zn(OH)_4}} = 7.0 \cdot 10^{-4}\,\frac{\mathrm{S{\cdot}m^2}}{\mathrm{mol}} \quad , \quad \Lambda_{\mathrm{K_2CO_3}} = 7.818 \cdot 10^{-3}\,\frac{\mathrm{S{\cdot}m^2}}{\mathrm{mol}} - 7.14 \cdot 10^{-7}\,\frac{\mathrm{S{\cdot}m^5}}{\mathrm{mol^2}} \cdot c_{\mathrm{K^+}} \,. \tag{S29}$$

The conductivity $\kappa_{\mathrm{KOH}}$ is experimentally determined and fitted by See et al. [14]. It is

$$\kappa_{\mathrm{KOH}} = K_1 w + K_2 T + K_3 T^2 + K_4 T w + K_5 T^2 w^{K_6} + K_7 \frac{T}{w} + K_8 \frac{w}{T} \,, \tag{S30}$$

with the weight percentage $w$ of potassium hydroxide in pure water

$$w = 100 \cdot \frac{c_{\mathrm{KOH}} M^{\mathrm{mol}}_{\mathrm{KOH}}}{c_{\mathrm{KOH}} M^{\mathrm{mol}}_{\mathrm{KOH}} + c_{\mathrm{H_2O}} M^{\mathrm{mol}}_{\mathrm{H_2O}}} \,. \tag{S31}$$

The coefficients $K_i$ of Eq. (S30) are listed in Table S3. The molar masses are $M^{\mathrm{mol}}_{\mathrm{H_2O}} = 18.015\,28 \cdot 10^{-3}\,\mathrm{kg{\cdot}mol^{-1}}$ and $M^{\mathrm{mol}}_{\mathrm{KOH}} = 56.105\,64 \cdot 10^{-3}\,\mathrm{kg{\cdot}mol^{-1}}$.

*S3.5. Transference Numbers*

The transference numbers are calculated from the mobilities at infinite dilution. Newman et al. show an application to binary electrolytes [18]. According to Ref. [2], the transference numbers are

$$t_{\beta_\mathrm{l}^{+-}} = \frac{c_{\beta_\mathrm{l}^{+-}} \left|z_{\beta_\mathrm{l}^{+-}}\right| \lambda_{\beta_\mathrm{l}^{+-}}}{\sum\limits_{\beta_\mathrm{l}^{+-}} c_{\beta_\mathrm{l}^{+-}} \left|z_{\beta_\mathrm{l}^{+-}}\right| \lambda_{\beta_\mathrm{l}^{+-}}} \,, \tag{S32}$$

with the ionic conductivities $\lambda_{\beta_\mathrm{l}^{+-}}$ from Table S4.

*S3.6. Permeability*

We present here the intrinsic permeability. The transformation to its superficial form is done by $B_\mathrm{l}^{\mathrm{sup}} = \phi B_\mathrm{l}^{\mathrm{in}}$, with the porosity $\phi = 1 - \varepsilon_\mathrm{s}$. We use the Kozeny-Carman equation [19, chap. 5.10] to describe single phase flow in disordered media. To describe a multi-phase flow, it is multiplied with the saturation $s_\mathrm{l} = \varepsilon_\mathrm{l}/\phi$.

$$B_\mathrm{l}^{\mathrm{in}} = s_\mathrm{l} \frac{\phi^2 d^2}{180(1-\phi)^2} = \frac{\varepsilon_\mathrm{l} \phi d^2}{180(1-\phi)^2} \,. \tag{S33}$$

*S3.7. Viscosity*

The viscosity of the electrolyte cannot be calculated exactly, since there is no formulation, depending on all the dissolved species. However, Siu et al. examine its dependence on the concentration of zincate in a potassium hydroxide solution [7] . It is

$$\eta_\mathrm{l} = 2.060 \cdot 10^{-3}\,\mathrm{Pa{\cdot}s} + 3.888 \cdot 10^{-4}\,\mathrm{Pa{\cdot}s} \cdot \frac{c_{\mathrm{Zn(OH)_4^{2-}}}}{c_{\mathrm{std}}} + 1.185 \cdot 10^{-5}\,\mathrm{hPa{\cdot}s} \cdot \left(\frac{c_{\mathrm{Zn(OH)_4^{2-}}}}{c_{\mathrm{std}}}\right)^2 \,. \tag{S34}$$

This formulation neglects the carbonate concentration, but it comes close enough to the used electrolyte.

| | value / $\frac{\mathrm{S{\cdot}m^2}}{\mathrm{mol}}$ | Reference |
|---|---|---|
| $\lambda_{\mathrm{K^+}}$ | $7.35 \cdot 10^{-3}$ | [16] |
| $\lambda_{\mathrm{OH^-}}$ | $1.98 \cdot 10^{-2}$ | [16] |
| $\lambda_{\mathrm{Zn(OH)_4^{2-}}}$ | $9.035 \cdot 10^{-3}$ | [17] |
| $\lambda_{\mathrm{CO_3^{2-}}}$ | $6.98 \cdot 10^{-3}$ | [16] |

Table S4: Ionic conductivities $\lambda_{\beta_\mathrm{l}^{+-}}$ at infinite dilution.

*S3.8. Leverett Function (Liquid)*

To calculate the liquid pressure, we use the Leverett function $J_l$, which has the form

$$J_l(s_l) = -c_1 \left[\sinh\left(c_2\left(s_l - s_i^*\right)\right) + c_3 \tan\left(\left(s_l - 0.5\right)\pi\right)\right] , \tag{S35}$$

With the liquid saturation $s_l = \varepsilon_l/(1 - \varepsilon_s)$. The first term describes the liquid pressure under normal conditions dependent on the saturation. The second term influences the pressure only if the saturation is close to zero or one. It is a modification to achieve more numerical stability by preventing $\varepsilon_l$ from reaching values smaller than zero or larger than one. The coefficients of Eq. (S35) are shown in Table S5. This Leverett function is motivated by measurements and simulations [20, 21].

| Domain | $c_1$ [Pa] | $c_2$ [1] | $c_3$ [1] | $s_i^*$ [1] |
|---|---|---|---|---|
| Anode | 1 | 6 | $1 \cdot 10^{-1}$ | $0.005 + 0.99 * \sqrt{\varepsilon_s}$ |
| Separator | 1 | 11 | $2 \cdot 10^{-1}$ | $0.95 + 0.04 * \sqrt{\varepsilon_s}$ |
| Cathode | 5 | 6 | $1 \cdot 10^{-1}$ | $0.005 + 0.99 * \sqrt{\varepsilon_s}$ |

Table S5: Domain parameters of the Leverett function Eq. (S35).

## S4. Reactions and Parameters

Our volume-averaged transport theory is coupled to reaction rates as described in Section 3.5. We model reaction rates by a consistent Butler-Volmer approach [22, 23],

$$j = 2 j_0 \sinh\left(\frac{1}{2}\frac{|z|\,F}{RT}\eta\right), \tag{S36}$$

with the exchange current density $j_0$, universal gas constant $R$, temperature $T$, the Faraday constant $F$, number of transferred electrons $z$, and the activation overpotential $\eta$. In the following, we briefly describe each reaction in our model (see Fig. 2).

*S4.1. Reaction I: Zinc Dissolution and Deposition*

We model zinc metal dissolution and deposition in the negative electrode into and from zincate ions in the electrolyte,

$$Zn + 4OH^- \leftrightharpoons Zn(OH)_4^{2-} + 2e^- . \tag{I}$$

The reaction rate is

$$j_I = 2k_I \sqrt{\frac{c_{s,OH^-}^4 c_{Zn(OH)_4^{2-}}}{c_{std}^5}} \sinh\left(\frac{F}{RT}\eta_a\right), \tag{S37}$$

with the kinetic prefactor $k_I$. As discussed by Stamm et al. [2], this value is two orders of magnitudes lower than the one measured on pure zinc [17, 24]. In commercial button cells, zinc anodes contain additives to reduce hydrogen evolution, which can decrease the pure theoretical value.

$$k_I = 1.8 \cdot 10^{-6}\,\text{mol}\cdot\text{m}^{-2}\cdot\text{s}^{-1} . \tag{S38}$$

The anode overpotential is

$$\eta_a = \Delta\phi_a - \Delta\phi_a^0 - \frac{RT}{2F}\ln\left(\frac{c_{Zn(OH)_4^{2-}} c_{std}^3}{c_{s,OH^-}^4}\right). \tag{S39}$$

$\Delta\phi_a = \phi_s - \phi_l$ is the electric potential difference between the electrode and the electrolyte. We measure potential against the standard hydrogen electrode and the standard half-cell potential $\Delta\phi_a^0 = -1.285\,\text{V}$ [2].

*S4.2. Reaction II: Zinc Oxide Precipitation*

The precipitation of zinc oxide takes place on the zinc metal surface forming a porous zinc oxide layer with porosity $(1 - \varepsilon_\mathrm{f})$ and $\varepsilon_\mathrm{f} = 0.95$ [2],

$$\mathrm{Zn(OH)_4^{2-}} \leftrightharpoons \mathrm{ZnO} + \mathrm{H_2O} + 2\mathrm{OH^-}. \tag{II}$$

The reaction rate is

$$j_\mathrm{II} = (1 - \varepsilon_\mathrm{f})^\mathrm{b} \frac{D_{\mathrm{Zn(OH)_4^{2-}}}}{\delta_{j_\mathrm{II}}} \left( c_{\mathrm{Zn(OH)_4^{2-}}} - c_\mathrm{sat} \right) , \tag{S40}$$

with the zinc oxide layer thickness $\delta_{j_\mathrm{II}} = 1 \cdot 10^{-6}\,\mathrm{m}$ and the Bruggemann coefficient $\mathrm{b} = 3.09$. The thermodynamic equilibrium of Eq. (S40) is determined by the zinc solubility or saturation concentration of zincate $c_\mathrm{sat}$. Sunu et al. measured [25],

$$\frac{c_\mathrm{sat}}{c_\mathrm{std}} = \begin{cases} -2.1 \cdot 10^{-1} + 9.75 \cdot 10^{-2} \frac{c_{\mathrm{K^+}}}{c_\mathrm{std}} + 1.25 \cdot 10^{-3} \frac{c_{\mathrm{K^+}}}{c_\mathrm{std}}^2 & \text{if } \frac{c_{\mathrm{K^+}}}{c_\mathrm{std}} > 2.097445176 \\ 0 & \text{else}. \end{cases} \tag{S41}$$

for a potassium hydroxide solution.

Zinc oxide does not precipitate on any material surface just above the saturation concentration of zincate $c_\mathrm{sat}$. A critical supersaturation of zincate has to be reached before zinc oxide can nucleate and grow [26]. We choose the critical concentration $c_\mathrm{crit} \approx 3.5 c_\mathrm{sat}$ [15, 27]. Our numerical implementation of the model developed by Stamm et al. is presented along the specific surface areas in Eq. (S15) [2] .

*S4.3. Reaction III: Oxygen Dissolution*

Oxygen dissolves from the gas phase into the electrolyte in the gas diffusion electrode (positive electrode).

$$\mathrm{O_2^g} \leftrightharpoons \mathrm{O_2^l}. \tag{III}$$

Based on the Hertz-Knudsen equation [2, 26, 28], we calculate the reaction rate

$$j_\mathrm{III} = \frac{p_{\mathrm{O_2^g}} \zeta}{c^*_{\mathrm{O_2^l}} \left( 2\pi M^\mathrm{mol}_{\mathrm{O_2}} RT \right)^{0.5}} \left( c^*_{\mathrm{O_2^l}} - c_{\mathrm{O_2^l}} \right) . \tag{S42}$$

The partial gas pressure of oxygen is denoted by $p_{\mathrm{O_2^g}}$, $M^\mathrm{mol}_{\mathrm{O_2}} = 31.9988 \cdot 10^{-3}\,\mathrm{kg{\cdot}mol^{-1}}$ is the molar mass of oxygen, and $c^*_{\mathrm{O_2^l}}$ is the solubility of oxygen in water. The latter one is calculated via Henry's law. The parameter $\zeta = 0.01$ is a phenomenological constant [2, 26]. It is the ratio of dissolved oxygen molecules to gaseous oxygen molecules hitting the gas-liquid phase boundary. The partial pressures represent ambient air, i.e., 20.942 % and 0.038 % of the standard pressure $p_\mathrm{std} = 1.013\,25 \cdot 10^5\,\mathrm{Pa}$ for oxygen and carbon dioxide, respectively. The solubility of gases in electrolyte is highly dependent on their partial pressures and the composition of the liquid. According to Weisenberger et al. we write

$$\frac{c^*_{\beta_\mathrm{g},0}}{c^*_{\beta_\mathrm{g}}} = 10^{K^\mathrm{S}_{\beta_\mathrm{g}}} , \tag{S43}$$

with the solubility in pure water $c^*_{\beta_\mathrm{g},0}$ and the Sechenov constant $K^\mathrm{S}_{\beta_\mathrm{g}}$ [29]. The first one is determined by Henry's law

$$c^*_{\beta_\mathrm{g},0} = p_{\beta_\mathrm{g}} H^\mathrm{cp}_{\beta_\mathrm{g}} . \tag{S44}$$

$p_{\beta_\mathrm{g}}$ is the partial pressure of the species $\beta_\mathrm{g}$ and $H^\mathrm{cp}_{\beta_\mathrm{g}}$ are the corresponding Henry's law constants [30]. They are

$$H^\mathrm{cp}_{\mathrm{O_2^g}} = 1.283 \cdot 10^{-5}\, \frac{\mathrm{mol}}{\mathrm{Pa{\cdot}m^3}} \quad , \quad H^\mathrm{cp}_{\mathrm{CO_2^g}} = 3.356 \cdot 10^{-4}\, \frac{\mathrm{mol}}{\mathrm{Pa{\cdot}m^3}} . \tag{S45}$$

The Sechenov constant is

$$K^\mathrm{S}_{\beta_\mathrm{g}} = \sum_{\beta_\mathrm{l}} \left( h_{\beta_\mathrm{l}} - h_{\beta_\mathrm{g}} \right) c_{\beta_\mathrm{l}} . \tag{S46}$$

The values of $h_{\beta_\mathrm{l}}$ and $h_{\beta_\mathrm{g}}$ are listed in Ref. [29] and are shown in Table S6.

| Liquid species | $h_{\beta_l}$ / m$^3$·mol$^{-1}$ |
|---|---|
| $H_2O$ | 0.0 |
| $K^+$ | $9.22 \cdot 10^{-2}$ |
| $OH^-$ | $8.39 \cdot 10^{-2}$ |
| $Zn(OH)_4^{2-}$ | $1.43 \cdot 10^{-1}$ |
| $CO_3^{2-}$ | $1.43 \cdot 10^{-1}$ |
| **Gaseous species** | $h_{\beta_g}$ / m$^3$·mol$^{-1}$ |
| $O_2^g$ | 0.0 |
| $CO_2^g$ | $-1.72 \cdot 10^{-2}$ |

Table S6: Solubility parameter for the calculation of the Sechenov constant (Eq. (S46)). We find no measurement for $h_{Zn(OH)_4^{2-}}$, so we choose it identical to $h_{CO_3^{2-}}$.

### *S4.4. Reaction IV: Oxygen Reduction and Evolution*

Dissolved oxygen is reduced to hydroxide at the electrolyte-GDE interface

$$\frac{1}{2}O_2^l + H_2O + 2e^- \leftrightharpoons 2OH^- \,. \tag{IV}$$

This reaction is expressed by a Butler-Volmer rate [31]. It is

$$j_{IV} = -2k_{IV}\frac{c_{OH^-}}{c_{std}}\sqrt[4]{\frac{c_{O_2^l}}{c_{std}^{O_2}}}\sinh\left(\frac{F}{RT}\eta_c\right), \tag{S47}$$

$$\eta_c = \Delta\phi_c - \Delta\phi_c^0 - \frac{RT}{2F}\ln\left(\sqrt{\frac{c_{O_2^l}}{c_{std}^{O_2}}}\frac{c_{std}^2}{c_{OH^-}^2}\right). \tag{S48}$$

The standard potential difference is $\Delta\phi_c^0 = 0.401$ V. The reaction constant is set to

$$k_{IV} = 3 \cdot 10^{-10}\,\text{mol·m}^{-2}\text{·s}^{-1} \,. \tag{S49}$$

It is in agreement with the measurements of Gyenge et al. for carbon based gas diffusion electrodes coated with manganese dioxide [32].

### *S4.5. Reaction V: Carbonation*

A major degradation mechanism for alkaline electrolytes is electrolyte carbonation. Atmospheric carbon dioxide dissolves and reacts to carbonate

$$CO_2 + 2OH^- \leftrightharpoons CO_3^{2-} + H_2O. \tag{V}$$

A model for this reaction was derived by Stamm et al. [2]. This reaction is actually a two-step process. First, the gaseous carbon dioxide is dissolved in the electrolyte, where it starts to diffuse away from the phase boundary. The second process is reaction (V), which is very fast [2]. The total reaction rate is given by

$$j_V = c_{CO_2}^* \sqrt{k_V D_{CO_2}}\,, \tag{S50}$$

with the solubility $c_{CO_2}^*$ of carbon dioxide in water (see Section S4.3) and its diffusion constant in the electrolyte $D_{CO_2} = 1.5 \cdot 10^{-9}\,\frac{m^2}{s}$. The reaction coefficient is

$$k_V = k_{OH^-}\frac{c_{OH^-}}{c_{std}}\,, \tag{S51}$$

with the reaction coefficient of the rate limiting process [33]

$$k_{OH^-} = 10^{(11.916-\frac{2383}{T})+\left(0.11c_{K^+}+0.11c_{OH^-}+0.17c_{CO_3^{2-}}\right)/c_{std}}\,. \tag{S52}$$

## S5. Validation of Implementation: 1D vs. 3D

Previously, we published a 1D model of zinc-air button cells, implemented in Matlab [2]. It utilizes the ode15i function as an underlying nonlinear implicit solver. To ensure a correct implementation of our 3D code in BEST (see Section 4.2), we compare simulation results of both codes. For that, we use the same geometrical setup, identical initial conditions, and an equivalent discretization in the through direction. The discretization is realized by a $(66, 1, 1) \times 1$ grid ((anode, separator, cathode) x-dir $\times$ radial discretization units).

We compare the two programs with a set of galvanostatic simulations at various currents. A detailed analysis of the simulation results shows that the spatial profiles of concentration and phase volume fractions match. Here, in Fig. S4, we compare the voltage profiles. We see that both codes, deliver results, which agree within the numerical accuracy, independent of the applied current. We conclude that our 3D code is correctly implemented.

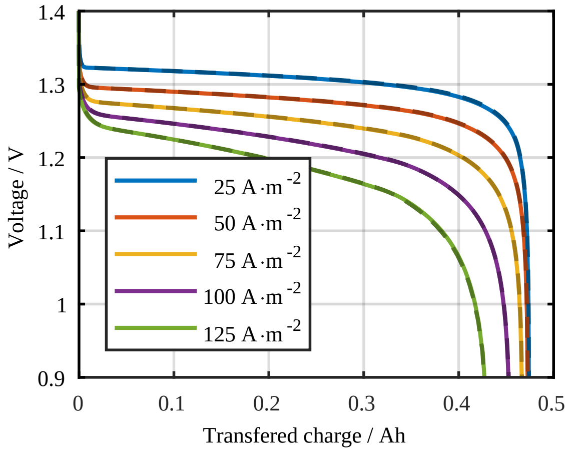


Figure S4: Comparison of 1D Matlab (dashed lines) [2] and 3D BEST simulations (solid lines). The voltage curves for all five currents coincide for 1D and 3D.

## S6. Determination of Optimal Grid Resolution

In this section, we examine the dependence of simulation results on the resolution of the computational grid. This is a special issue in simulations of local volume-averaged models. In general it holds that the better the resolution, the better the results. But an important assumption of local volume-averaging is that the averaging volume must be larger than the typical length scale of the underlying structure. Because the typical size of the zinc particles is on the order of a few tens of micro meters, very fine resolutions would be contradictory. We discuss now that quite coarse resolutions are numerically sufficient.

This is visualized in Fig. S5a and b for the cell voltage and the distribution of $\varepsilon_{Zn}/\varepsilon_{ZnO}$. The coarsest grid is not sufficient to reproduce the cell voltage, or an adequate volume fraction profile. It shows numerically induced nucleation effects at $\sim 30\,\%$ SOC as a step in the discharge voltage. A resolution of $(30, 1, 3) \times 4$ is already enough to capture the most important effects properly. A further increase of the resolution shows only minor effects on the voltage profile. The distributions of the phases and the concentrations are simulated properly with $(50, 2, 6) \times 10$ discretization units. We choose this resolution for cycling simulations and the resolution $(70, 3, 9) \times 20$ for discharge simulations.

## S7. Solid Phase Movement

In order to examine the mechanism of solid phase movement, we plot the reaction rate of zinc dissolution and formation (reaction I) in Fig. S6. A positive value means dissolution and a negative one formation of Zn. We observe

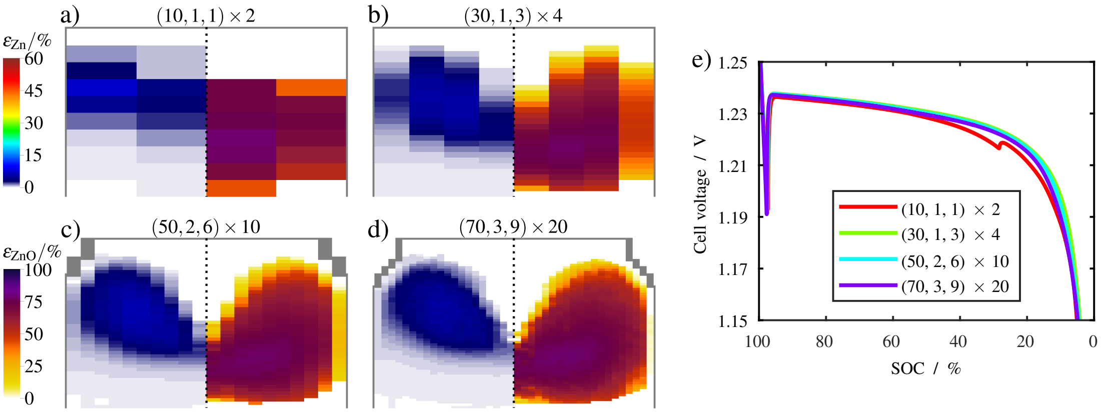


Figure S5: Analysis of the volume fraction distribution and cell voltage on the discretization during discharge. The left half cells shows the zinc and the right one the zinc oxide volume fractions. The resolution is specified in the form: (anode, separator, cathode) x-dir × radial discretization units.

that Zn dissolves and forms predominantly near the cathode. Comparing dissolution and deposition, however, Zn formation occurs slightly closer to the lid than Zn dissolution. Therefore, charging and discharging do not exactly balance each other and a phase-shift to the lid remains.

We quantify the solid-phase-movement with the center-of-volume

$$\bar{\bar{x}}_i = \frac{1}{\int \varepsilon_i(x)\mathrm{d}x} \cdot \int x\varepsilon_i(x)\mathrm{d}x. \tag{S53}$$

The dynamics of the center-of-volume $\bar{\bar{x}}_s$ of all solid phases is plotted in Fig. 6b and discussed in the main text.

We quantify agglomeration with the width of ZnO,

$$\Delta x_i = 2\sqrt{3} \cdot \sigma_i, \tag{S54}$$

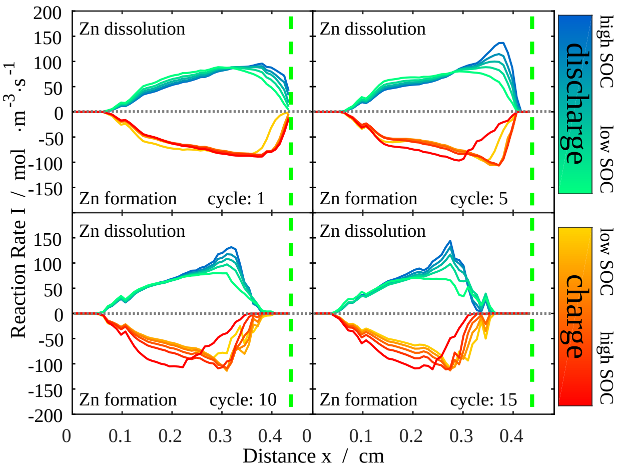


Figure S6: Examination of the solid phase movement by the zinc precipitation and dissolution behavior. The plot shows a radial projection of the reaction rate (I) for different cycle numbers. The dashed green line represents the separator. $T = 298.15$ K; $\boldsymbol{j} = 100$ A·m$^{-2}$

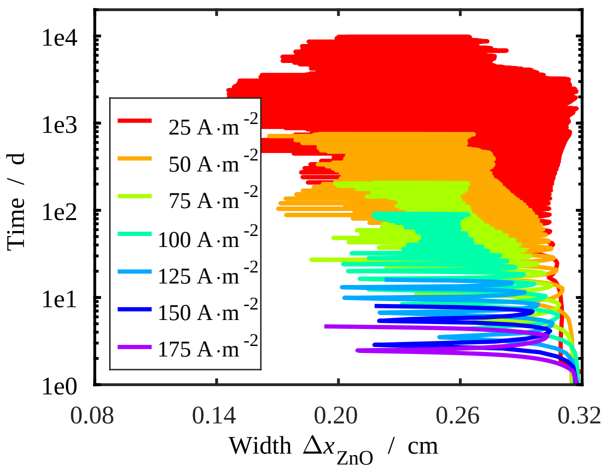


Figure S7: Width of solid ZnO $\Delta x_{\mathrm{ZnO}}$ during repeated discharge and charge (see Eq. (S54)). ($T = 298.15\,\mathrm{K}$)

where $\sigma$ is the standard deviation,

$$\sigma_i = \sqrt{\frac{1}{\int \varepsilon_i(x)\mathrm{d}x} \int \varepsilon_i(x) x^2 \mathrm{d}x - \bar{\bar{x}}_i^2}. \tag{S55}$$

$\Delta x_{\mathrm{ZnO}}$ is plotted in Fig. S7. The width of solid ZnO increases during discharge and decreases during charge. This yields a zigzag behavior of the overall graph. Once the ZnO profile shrinks from initially $\Delta x_{\mathrm{ZnO}} = 3.2\,\mathrm{mm}$ to $\Delta x_{\mathrm{ZnO}} \lesssim 2\,\mathrm{mm}$, the cell fails for high current densities. For low current densities, the situation is more complex as ZnO dissolution is less critical. This demonstrates the mechanism of ZnO agglomeration and its relevance for cycle-life limitation.

## S8. Reaction and Transport Kinetics Optimization

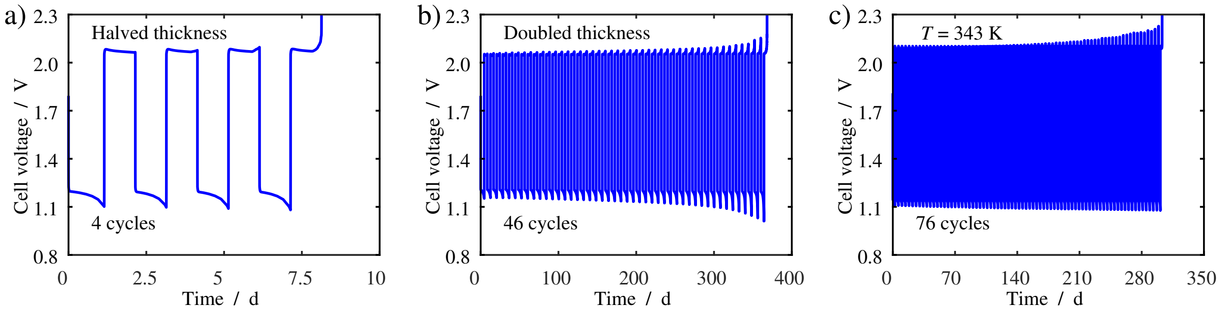


Figure S8: Improving the cycle-life by varying the anode geometry or the temperature. The thickness (x-dir) of the anode is varied in (a) and (b). The temperature is increased to $T = 343.15\,\mathrm{K}$ in (c).

In order to improve the cycle-life we analyze two further setups. Firstly, we alter the thickness (x-dir) of the anode, which enhances the total specific surface area for the simulations. Secondly, we increase the temperature to $T = 343.15\,\mathrm{K}$, which enhances the electrolyte transport processes by a factor of 2. Thus, the concentration gradients along the through direction are more homogeneous, which slows down the movement of the solid phases. We use a linear profile for the initial zinc distribution (see Fig. 7h) with 2 % zinc oxide. The charge-discharge protocol corresponds to protocol **A** (see Table 2).

The anode thickness is halved in Fig. S8a and doubled in Fig. S8b. This modifies the cell capacity by a factor of two. We see that halving the thickness reduces the number of cycles. The reason is the reduced total surface area of zinc oxide. Therefore, the zincate concentration depletes earlier. Doubling the thickness has exactly the opposite effect. Because of the increased total zinc oxide surface area, 46 cycles are achieved. This is 1.4 times more than for the baseline reference geometry.

For Fig. S8c, we enhance electrolyte transport by increasing the temperature. Without decreasing the charging current, we achieve 76 cycles. However, the increased temperature leads to a reduced efficiency. Dependent on the application, a trade-off has to be found between cycle-life and efficiency, when adjusting the temperature. Thus, this is a very promising strategy to extend cycle-life.

## References


[1] T. Arlt, D. Schröder, U. Krewer, I. Manke, In operando monitoring of the state of charge and species distribution in zinc air batteries using X-ray tomography and model-based simulations, Phys. Chem. Chem. Phys. 16 (40) (2014) 22273–22280. doi:10.1039/C4CP02878C.

[2] J. Stamm, A. Varzi, A. Latz, B. Horstmann, Modeling nucleation and growth of zinc oxide during discharge of primary zinc-air batteries, Journal of Power Sources 360 (2017) 136–149. doi:10.1016/j.jpowsour.2017.05.073.

[3] Q. C. Horn, Y. Shao-Horn, Morphology and Spatial Distribution of ZnO Formed in Discharged Alkaline Zn/$MnO_2$ AA Cells, Journal of The Electrochemical Society 150 (5) (2003) A652–A658. doi:10.1149/1.1566014.

[4] I. Manke, J. Banhart, A. Haibel, A. Rack, S. Zabler, N. Kardjilov, A. Hilger, A. Melzer, H. Riesemeier, In situ investigation of the discharge of alkaline Zn-$MnO_2$ batteries with synchrotron x-ray and neutron tomographies, Applied Physics Letters 90 (21) (2007) 214102. doi:10.1063/1.2742283.

[5] P. Miller, The Electrical Conductivity of Zinc Oxide, Physical Review 60 (12) (1941) 890–895. doi:10.1103/PhysRev.60.890.

[6] Metal properties table, https://www.tibtech.com/conductivite.php?lang=en_US . Last visited 2019-01-08.

[7] S. Siu, J. W. Evans, Density and Viscosity Measurements of Zincate/KOH Solutions, Journal of The Electrochemical Society 144 (4) (1997) 1278–1280. doi:10.1149/1.1837583.

[8] E.-A. Zen, Partial molar volumes of some salts in aqueous solutions, Geochimica et Cosmochimica Acta 12 (1-2) (1957) 103–122. doi:10.1016/0016-7037(57)90022-4.

[9] R. N. Bhatia, K. E. Gubbins, R. D. Walker, Mutual diffusion in concentrated aqueous potassium hydroxide solutions, Trans. Faraday Soc. 64 (1968) 2091–2099. doi:10.1039/TF9686402091.

[10] C. E. May, H. E. Kautz, Determination of the Zincate Diffusion Coefficient and its Application to Alkaline Battery Problems, NASA STI/NASA Technical Report (1978).
URL https://ntrs.nasa.gov/archive/nasa/casi.ntrs.nasa.gov/19780011705.pdf

[11] A. H. G. Cents, Mass transfer and hydrodynamics in stirred gas-liquid-liquid contactors, Phd thesis, University of Twente (2003).

[12] R. E. Zeebe, On the molecular diffusion coefficients of dissolved $CO_2$, $HCO_3^-$, and $CO_3^{2-}$ and their dependence on isotopic mass, Geochimica et Cosmochimica Acta 75 (9) (2011) 2483–2498. doi:10.1016/J.GCA.2011.02.010.

[13] R. E. Davis, G. L. Horvath, C. W. Tobias, The Solubility and Diffusion Coefficient of Oxygen in Potassium Hydroxide Solutions, Electrochimica Acta 12 (297) (1967) 287–297. doi:10.1016/0013-4686(67)80007-0.

[14] D. M. See, R. E. White, Temperature and concentration dependence of the specific conductivity of concentrated solutions of potassium hydroxide, Journal of Chemical & Engineering Data 42 (6) (1997) 1266–1268. doi:10.1021/je970140x.

[15] M.-B. Liu, B. R. Faulds, G. M. Cook, N. P. Yao, Conductivity of KOH Electrolyte Supersaturated with Zincate, Journal of The Electrochemical Society 128 (9) (1981) 2049–2052. doi:10.1149/1.2127187.

[16] J. A. Dean, N. A. Lange, Lange's Handbook of Chemistry, 15th Edition, McGRAW-HILL, INC, New York, NY, USA, 1999.

[17] W. G. Sunu, D. N. Bennion, Transient and Failure Analyses of the Porous Zinc Electrode, Journal of The Electrochemical Society 127 (9) (1980) 2007–2016. doi:10.1149/1.2130054.

[18] J. S. Newman, K. E. Thomas-Alyea, Electrochemical systems, 3rd Edition, J. Wiley, Hoboken, NJ, USA, 2004.

[19] J. Bear, Dynamics of Fluids in Porous Media, 1st Edition, Elsevier, New York, NY, USA, 1972.

[20] T. Danner, B. Horstmann, D. Wittmaier, N. Wagner, W. G. Bessler, Reaction and transport in Ag/$Ag_2O$ gas diffusion electrodes of aqueous $LiO_2$ batteries: Experiments and modeling, Journal of Power Sources 264 (2014) 320–332. doi:10.1016/j.jpowsour.2014.03.149.

[21] T. Danner, S. Eswara, V. P. Schulz, A. Latz, Characterization of gas diffusion electrodes for metal-air batteries, Journal of Power Sources 324 (2016) 646–656. doi:10.1016/j.jpowsour.2016.05.108.

[22] A. Latz, J. Zausch, Thermodynamic derivation of a Butler-Volmer model for intercalation in Li-ion batteries, Electrochimica Acta 110 (2013) 358–362. doi:10.1016/j.electacta.2013.06.043.

[23] M. Z. Bazant, Theory of Chemical Kinetics and Charge Transfer based on Nonequilibrium Thermodynamics, Accounts of Chemical Research 46 (5) (2013) 1144–1160. doi:10.1021/ar300145c.

[24] E. Deiss, F. Holzer, O. Haas, Modeling of an electrically rechargeable alkaline Zn-air battery, Electrochimica Acta 47 (25) (2002) 3995–4010. doi:10.1016/S0013-4686(02)00316-X.

[25] W. G. Sunu, Transient and Failure Analyses of Porous Zinc Electrodes, Phd thesis, University of California, Los Angeles (1978).

[26] B. Horstmann, T. Danner, W. G. Bessler, Precipitation in aqueous lithium-oxygen batteries: a model-based analysis, Energy & Environmental Science 6 (4) (2013) 1299–1314. doi:10.1039/c3ee24299d.

[27] M.-B. Liu, G. M. Cook, N. P. Yao, Passivation of Zinc Anodes in KOH Electrolytes, Journal of The Electrochemical Society 128 (8) (1981) 1663–1668. doi:10.1149/1.2127707.

[28] I. W. Eames, N. J. Marr, H. Sabir, The evaporation coefficient of water: a review, International Journal of Heat and Mass Transfer 40 (12) (1997) 2963–2973. doi:10.1016/S0017-9310(96)00339-0.

[29] S. Weisenberger, A. Schumpe, Estimation of gas solubilities in salt solutions at temperatures from 273 K to 363 K, AIChE Journal 42 (1) (1996) 298–300. doi:10.1002/aic.690420130.

[30] R. Sander, Compilation of Henry's law constants (version 4.0) for water as solvent, Atmos. Chem. Phys 15 (2015) 4399–4981. doi:10.5194/acp-15-4399-2015.

[31] D. Eberle, B. Horstmann, Oxygen Reduction on Pt(111) in Aqueous Electrolyte: Elementary Kinetic Modeling, Electrochimica Acta 137 (2014) 714–720. doi:10.1016/J.ELECTACTA.2014.05.144.

[32] E. L. Gyenge, J.-F. Drillet, The Electrochemical Behavior and Catalytic Activity for Oxygen Reduction of $MnO_2$/C-Toray Gas Diffusion Electrodes, Journal of The Electrochemical Society 159 (2) (2012) F23–F34. doi:10.1149/2.061202jes.

[33] R. Pohorecki, W. Moniuk, Kinetics of reaction between carbon dioxide and hydroxyl ions in aqueous electrolyte solutions, Chemical Engineering Science 43 (7) (1988) 1677–1684. doi:10.1016/0009-2509(88)85159-5.
